# Supplementary material for: Empirical Mass and Radius Relations for Main-sequence Stars from Detached Eclipsing Binaries
Source: arXiv:2611.28229 source file (2026-11-20)
Supplement: Supplementary file 1 [file appendix_parsec_comparison_table.tex]

\begin{deluxetable}{lccccc}[t]
\tablecaption{\tablecaptiontext}
\tablehead{
\colhead{Term} & \colhead{EB} & \colhead{MIST} & \colhead{Shift} & \colhead{PARSEC} & \colhead{Shift} \\
\colhead{} & \colhead{} & \colhead{} & \colhead{[$\sigma$]} & \colhead{} & \colhead{[$\sigma$]}
}
\startdata
${\rm const}$ & $0.1692\pm0.0009$ & $0.1591\pm0.0005$ & $-9.8$ & $0.1567\pm0.0005$ & $-12.2$ \\
$X$ & $0.63\pm0.01$ & $0.687\pm0.008$ & $+3.6$ & $0.662\pm0.009$ & $+1.9$ \\
$Y$ & $-0.593\pm0.004$ & $-0.589\pm0.002$ & $+1.0$ & $-0.590\pm0.002$ & $+0.8$ \\
$Z$ & $0.067\pm0.003$ & $0.083\pm0.002$ & $+4.0$ & $0.070\pm0.002$ & $+0.7$ \\
$X^2$ & $0.19\pm0.02$ & $0.18\pm0.01$ & $-0.3$ & $0.20\pm0.02$ & $+0.7$ \\
$Y^2$ & $0.047\pm0.009$ & $0.076\pm0.006$ & $+2.7$ & $0.073\pm0.005$ & $+2.5$ \\
$Z^2$ & $0.007\pm0.002$ & $0.013\pm0.002$ & $+2.1$ & $0.006\pm0.002$ & $-0.2$ \\
$Y Z$ & $-0.028\pm0.005$ & $-0.026\pm0.005$ & $+0.3$ & $-0.020\pm0.005$ & $+1.1$ \\
\hline
RMS [dex] & $0.0161$ & $0.0104$ & \nodata & $0.0104$ & \nodata \\
\enddata
\end{deluxetable}
